# Supplementary material for: VisCoder2: Building Multi-Language Visualization Coding Agents
Source: arXiv:2510.23642 source file (2026-04-07)
Supplement: Supplementary file 1 [file llm_usage.tex]

\newpage
\clearpage

\section{LLM Usage}
Large Language Models (LLMs) were used to assist with language editing and polishing of the manuscript. Specifically, we used an LLM to refine wording, improve readability, and enhance clarity in several sections.

The LLM was not involved in research ideation, methodology, data analysis, or experimental design. All technical ideas, analyses, and conclusions were developed and validated by the authors; the tool was limited to editorial support.

The authors take full responsibility for the content of the manuscript, including any text edited with LLM assistance. We verified suggested edits for accuracy and originality, ensured compliance with ethical guidelines, and noted that LLMs are not listed as authors. We disclose this usage in accordance with ICLR’s policies on LLM assistance and attribution.
